# Supplementary material for: Mava: a research library for distributed multi-agent reinforcement learning in JAX
Source: arXiv:2107.01460 source file (2023-12-15)
Supplement: Supplementary file 1 [file appendix.tex]

% Note: in this sample, the section number is hard-coded in. Following
% proper LaTeX conventions, it should properly be coded as a reference:

%In this appendix we prove the following theorem from
%Section~\ref{sec:textree-generalization}:

\section{Code API and Usage} \label{app:api}
Figure~\ref{fig:apisnippet} shows an example of the code usage demonstrating the simplicity and modularity of the API. This code snippet shows the main steps to run \me with \qdax, those steps being (i) instantiating an object from the class \me (ii) computing the centroids that will be used to define the grid that is to store the solutions produced by the algorithm (iii) initializing the algorithm, which will initialize the repertoire as well as the state of the emitter (iv) running iterations of the update function of \me, natively implemented in the class. Interestingly, all it takes to run \pgame or \cmame is to change the type of emitter defined when instantiating the \me object on the first line of the code snippet.

For additional illustrations of the API, we strongly encourage the reader to try the examples proposed in \qdax: we wrote example notebooks\footnote{\url{https://github.com/adaptive-intelligent-robotics/QDax/tree/main/examples}} for most algorithms implemented. This should help any user to get started with the library and should also illustrate how to use the library to extend the implemented algorithms for research purpose.

\begin{figure*}[ht!]
    \centering
    \includegraphics[width=1.0\textwidth]{images/qdax_api_example.png}
    \caption{Code snippet demonstrating the API of \qdax on a simple example: \me used to solve the arm task. User can get their first experiment running with only a few lines of code. Additionally, it only takes a few updates to change the type of algorithm running on the same task.}
    \label{fig:apisnippet}
    \vspace*{-0.3cm}
\end{figure*}

\section{Implemented algorithms} \label{app:algs}
The main algorithms implemented in \qdax are summarized in table~\ref{table:qdaxalgorithms_2}. This table provides the name of the algorithm, the broader categories of algorithms that the algorithm belongs to and the reference of the algorithm.

\begin{table} %[ht!]
    \begin{center}
    \begin{tabular}{lcc}
        \toprule
        \textbf{Algorithm} & \textbf{Categories} & \textbf{References} \\
        \midrule
        \me &  \qd & \citet{mouret2015illuminating}\\
        \cvtme &  \qd & \citet{vassiliades2017using}\\
        \midrule
        \cmame &  \qd, Evolution Strategies & \citet{fontaine2020covariance}\\
        \mees &  \qd, Evolution Strategies & \citet{colas2020scaling}\\
        \midrule
        \pgame &  \qd, \rl & \citet{nilsson2021policy}\\
        \qdpg &  \qd, \rl & \citet{pierrot2021diversity}\\
        \midrule
        \diayn &  Skill Discovery, \rl & \citet{eysenbach2018diversity}\\
        \dads &  Skill Discovery, \rl & \citet{sharma2020dads}\\
        \smerl &  Skill Discovery, \rl & \citet{kumar2020smerl}\\
        \midrule
        \omgmega &  Differentiable \qd & \citet{fontaine2021differentiable}\\
        \cmamega &  Differentiable \qd & \citet{fontaine2021differentiable}\\
        \midrule
        \mome &  Multi Objective, \qd & \citet{pierrot2022multi}\\
        \nsga &  Multi Objective & \citet{deb2002nsga2}\\
        \spea &  Multi Objective & \citet{zitzler2001spea2}\\
        \midrule
        \pbt & Population Based, RL & \citet{jaderberg2017pbt}\\
        \mepbt & Population Based, QD, RL & \citet{pierrot2023evolving}\\
        \bottomrule

    \end{tabular}
    \end{center}
    \caption{Main algorithms implemented in \qdax. This table also reports the general category of algorithms each method belongs to, as well as the paper that introduced the algorithm.}
    \label{table:qdaxalgorithms_2}
\end{table}

\qdax contains state-of-the-art \qd algorithms and numerous methods related to Neuroevolution, Skill Discovery, Population-Based learning and Multi-Objective optimization. 
In particular, \qdax provides the implementation of \me~\citep{mouret2015illuminating}, \cvtme~\citep{vassiliades2017using} - corresponding to general \qd methods -, \cmame~\citep{fontaine2020covariance}, \mees~\citep{colas2020scaling} - described as \qd with Evolution Strategies - , \pgame~\citep{nilsson2021policy, flageat2022empirical}, \qdpg~\citep{pierrot2021diversity} - which are \qd methods with policy gradients, often referred to as \qdrl - , \diayn~\citep{eysenbach2018diversity}, \dads~\citep{sharma2020dads}, \smerl~\citep{kumar2020smerl} - popular methods in \rl for Skill Discovery -, \omgmega, \cmamega~\citep{fontaine2021differentiable} - Differentiable \qd - , \mome~\citep{pierrot2022multi}, \nsga, \spea - the reference approaches for Multi-Objective optimization -. All those methods have similar API and can be evaluated on popular tasks. Furthermore, they all take advantage from the speed-up enabled by just-in-time compilation in Jax, making them extremely fast and scalable.

\section{Benchmark Results} \label{app:results}
This section provides numerous results from the algorithms present in \qdax over several benchmarks tasks available in the library.  These results can give the reader an idea of the metrics and time performance expected when using \qdax. Note that metrics performance are validated against the one reported along original implementations of the algorithms. The reported experiments are taken from \citet{chaluboige2022neuroevolution} and were run with a single Quadro RTX 4000 GPU.

The results presented relate to seven tasks from the \brax \rl tasks implemented in \qdax. These tasks are benchmark \qdrl tasks used to assess Neuroevolution algorithms~\citep{chalumeau2022assessing, flageat2022benchmarking}. We refer to them as \antuni, \hcuni, \walkeruni, \anttrap, \antmaze and \ptmaze. Those can be visualized on \autoref{fig:env_viz}. For more details about the hyper-parameters used, please refer to~\citep{chaluboige2022neuroevolution}. 

For a representative comparison between \qd algorithms and Deep \rl methods such as \smerl, which do not actively have a population of policies or an archive, a passive archive is used to compute metrics like \qd score in those results. Given that there is only a single latent conditioned policy, during training SMERL policy is evaluated by sampling latent codes and recording their trajectories. Behavior descriptors can be extracted from these trajectories, which can then be used for addition to the passive archive. This allows to use similar metrics such as the coverage and \qd score when comparing \qd and Skill Discovery \rl methods.

To demonstrate the speed of our implementations, \autoref{table:training_step} reports the number of training steps achieved in two hours by the implementation of \qdax on a single GPU. \autoref{fig:qd_metrics_step} reports the evolution of fitness, QD score and coverage along time of the algorithms \smerl, \me and \pgame on the seven tasks mentioned above. We also report the evolution of those metrics along environments interactions on \autoref{fig:qd_metrics_step}. Finally, \autoref{fig:final_grids} shows the archives of resulting policies from the different algorithms where each cell corresponds to a policy and different behaviors.

%\begin{table} %[ht!]
%    \begin{center}
%    \begin{tabular}{lc}
%        
%        \toprule
%        \textbf{Algorithm} & \textbf{Environments steps} \\
%        \midrule
%    
%        \smerl & $1.0 \times 10^7$ \\
%        \diayn & $1.0 \times 10^7$ \\
%        \dads & $8.5\times 10^6$ \\
%        \pgame & $1.8\times 10^8$ \\
%        \me & $1.6 \times10^9$ \\
%        \bottomrule
%    
%    \end{tabular}
%    \end{center}
%    \caption{Number of training steps carried out (on average) during two hours of training by the various methods under study. Averaged over seven \brax tasks of \qdax.}
%    \label{table:training_step}
%\end{table}

\begin{table} %[ht!]
    \begin{center}
    \begin{tabular}{lccccc}
        
        \toprule
        %\textbf{Environment} & \textbf{AntOmni} & \textbf{AntUni} & \textbf{AntMaze} & \textbf{AntTrap} & \textbf{HalfcheetahUni} & \textbf{PointMaze} & \textbf{Walker2dUni} \\
        \textbf{Environment} & \me & \pgame & \smerl & \dads & \diayn \\
        \midrule
        \textbf{Ant Omni} & $1.7 \times 10^9$ & $1.85 \times 10^8$ & $1.01 \times 10^7$ & $8.9 \times 10^6$ & $1.01 \times 10^7$ \\
        \textbf{Ant Uni} & $2.45 \times 10^9$ & $1.9 \times 10^8$ & $1.0 \times 10^7$ & $7.8 \times 10^6$ & $9.97 \times 10^6$ \\
        \textbf{Ant Maze} & $1.05 \times 10^9$ & $1.7 \times 10^8$ & $7.09 \times 10^6$ & $8.62 \times 10^6$ & $9.70 \times 10^6$ \\
        \textbf{Ant Trap} & $1.08 \times 10^9$ & $1.3 \times 10^8$ & $9.81 \times 10^6$ & $8.46 \times 10^6$ & $9.73 \times 10^6$ \\
        \textbf{Halfcheetah Uni} & $9.83 \times 10^8$ & $1.39 \times 10^8$ & $1.08 \times 10^7$ & $8.43 \times 10^6$ & $1.07 \times 10^7$ \\
        \textbf{Point Maze} & $2.41 \times 10^9$ & $3.01 \times 10^8$ & $1.09 \times 10^7$ & $9.70 \times 10^6$ & $1.07 \times 10^7$ \\
        \textbf{Walker2d Uni} & $1.95 \times 10^9$ & $2.40 \times 10^8$ & $1.11 \times 10^7$ & $8.94 \times 10^6$ & $1.11 \times 10^7$ \\
        \midrule
        \textbf{Average} & $1.66 \times 10^9$ & $1.93 \times 10^8$ & $9.97 \times 10^6$ & $8.70 \times 10^6$ & $1.03 \times 10^7$ \\
        \bottomrule
    
    \end{tabular}
    \end{center}
    \caption{Number of training steps carried out during two hours of training by the various methods under study on seven \brax tasks of \qdax. Averaged over 5 seeds.}
    \label{table:training_step}
\end{table}

\begin{figure} %[h!]
    \centering
    \includegraphics[width=0.9\textwidth]{images/environments_benchmark.png}
    \caption{Visualisation of the environments used to show the performances of our implementations of \smerl, \pgame and \me. Diagram is adapted from \citet{chaluboige2022neuroevolution, flageat2022benchmarking, chalumeau2022assessing}}
    \label{fig:env_viz}
    %\vspace*{-0.3cm}
\end{figure}

\begin{figure} %[h!]
    \centering
    \includegraphics[width=0.9\textwidth]{images/metrics_along_time_qdax.png}
    \caption{Evolution of the maximum fitness, coverage and \qd score along environment interactions, during a training phase. Reports algorithms \smerl, \pgame and \me  on 2 hours of training.}
    \label{fig:qd_metrics_time}
    %\vspace*{-0.3cm}
\end{figure}

\begin{figure} %[h!]
    \centering
    \includegraphics[width=0.9\textwidth]{images/metrics_along_steps_qdax.png}
    \caption{Evolution of the maximum fitness, coverage and \qd score along environment interactions, during a training phase. Reports \smerl on $10^7$ timesteps and \pgame and \me on $10^8$ timesteps.}
    \label{fig:qd_metrics_step}
    %\vspace*{-0.3cm}
\end{figure}

\begin{figure} %[h!]
    \centering
    \includegraphics[width=0.8\textwidth]{images/qdax_journal_paper_grids.png}
    \caption{Final grids obtained on 6 \brax environments with \qdax implementations. For \anttrap, \antmaze, \ptmaze and \antomni, the behavior descriptor is the final {x, y} position. For \walkeruni and \hcuni, it is the proportion of contact time of the feet on the ground. Reports \smerl, \pgame and \me after two hours of training.}
    \label{fig:final_grids}
    %\vspace*{-0.3cm}
\end{figure}

\section{Fast implementations}
\label{app:fast}

\qdax is a package written in \jax, hence all the implementations can be just-in-time compiled (jit) and run on hardware accelerators like GPUs and TPUs with no code overhead. This combines simplicity and efficiency, making \qdax particularly suitable for practitioners that do not have access to large compute resources. In this section, we put ourselves in the situation of a practitioner that has a machine with an affordable GPU and wants to use existing available open-source implementations by just installing and running them.

We consider a few open-source implementations of libraries and algorithms which runtime-performance is reported in a paper, reported by its authors, or by simply running the implementation to compare the runtime-performance to the one that someone can expect by running \qdax on an affordable GPU (Quadro RTX 4000).

For \pgame, we compare \qdax implementation with the only other available open-source implementation which is the provided author implementation\footnote{\url{https://github.com/ollenilsson19/PGA-MAP-Elites}}. The author implementation utilizes PyTorch as its deep learning framework. It also uses multiprocessing over CPU devices to handle its environment evaluation and is not directly compatible with GPUs even for training the networks via gradient descent. Hence, to exploit this implementation effectively, a large number of CPUs is required, which is not an option for most practitioners. The original implementation requires approximately 36 hours to perform a run of $10^9$ steps with 36 CPUs, which corresponds to $2.8 \times 10^7$ steps an hour. Our implementation of \pgame achieves $10^8$ steps an hour. Hence, a practitioner can perform runs of \pgame in a few hours on his computer instead of several days.

For \qdpg, we compare the runtime performance of \qdax's implementation with results reported by the authors of the algorithm. The author implementation is not open-source but they report that with 1 GPU and a dozen CPUs, their implementation can do $10^8$ steps in 15 hours on \anttrap. In \qdax, \qdpg can do the same on 3 hours, hence a speed-up of a factor 5.  

For \mees, we compare our implementation with the original implementation\footnote{\url{https://github.com/uber-research/Map-Elites-Evolutionary}}. This implementation requires large computing clusters to be efficient: results reported in the paper~\citep{colas2020scaling} use 1000 CPUs, which makes it completely unusable for most practitioners. Our implementation can be run on a simple GPU with a few CPUs and still match the runtime performance. The original implementation was reported to perform $6 \times 10^8$ environment steps an hour ($3 \times 10^{10}$ in two days for the \antmaze experiment). Our implementation performs $4 \times 10^8$ steps an hour.

For \me, the reader should refer to \citet{lim2022accelerated} for a thorough analysis of the performance to be expected in \qdax.
